# Supplementary material for: Boosting Feedback Efficiency of Interactive Reinforcement Learning by Adaptive Learning from Scores
Source: arXiv:2307.05405 source file (2023-08-06)
Supplement: Supplementary file 1 [file 06_appendix.tex]

\appendix
\begin{center}{\bf {\LARGE Appendix}}
\end{center}

\section{Experimental Details} \label{app:state_entropy}

\subsection{Policy training}
The poicy learning part of our code is built on the publicly released implementation repository of the off-policy RL algorithm SAC~\footnote{https://github.com/pranz24/pytorch-soft-actor-critic}. In the experiments of our approach and original SAC, we share the exact same hyperparameters across all tasks in different environments (Mujoco, Metaworld and RLBench) as shown in Table~\ref{table:hyperparameters_sac}.

\begin{table}[h!]

\centering
\begin{tabular}{l|l}
\toprule
\textbf{Hyperparameter} & \textbf{Value}\\
\midrule
Optimizer &Adam\\
Learning rate & 0.0003\\
Discount $\gamma$ &  0.99\\
Replay buffer size & $10^6$\\
Hidden layers (all networks) & 2\\
Hidden units per layer & 256\\
Samples per minibatch & 256\\
Nonlinearity & ReLU\\
Target smoothing coefficient $\tau$& 0.005\\
Target update interval & 1\\
Gradient steps & 1\\
\bottomrule
\end{tabular}
\caption{Hyperparameters for policy learning. In all experiments we use the same set of hypermaraters.}
\label{table:hyperparameters_sac}
\end{table}

\begin{table}[h!]

\centering
\begin{tabular}{l|l}
\toprule
\textbf{Hyperparameter} & \textbf{Value}\\
\midrule
Optimizer &Adam\\
Learning rate & 0.001\\
Input type &  $(s,a)$\\
Hidden layers (all networks) & 3\\
Hidden units per layer & 256\\
Samples per minibatch & 128\\
Nonlinearity & LeakyReLU\\
Priority weight $\beta$& 3\\
Adaptive coefficient $\alpha^\prime$ & 2\\
Scoring range & 0-12\\
\bottomrule
\end{tabular}
\caption{Hyperparameters for reward learning. In all experiments we share the same hyperparamters.}
\label{table:hyperparameters_reward}
\end{table}

\subsection{Reward training}
We model the reward function in our approach as a three-layer neural network. We also keep the hypermaraters for reward training unchanged in all experiments, and they are shown in Table~\ref{table:hyperparameters_reward}. For the experiments using correct scores, we set the threshold as $k=0.2$, if the difference of scores of two trajectories is less than 0.2, we consider them to be equally good and assign the label $\mu=0.5$ for both of them. For the experiments using noisy scores, we set the score precision to 0.5, e.g., 3.5, 6.0, 8.5. 

% \section{Customized Behavior}
% To verify that our method enables the agent to act according to the teacher's preferences, in the PushButton task from the RLBench environment, we model two scripted teachers to train pushing the button vertically by gripper tip and horizontally by gripper side respectively. Figure~\ref{figure5} shows the behaviors of the trained policy, demonstrating that our approach can infer user's underlying intent.

% \begin{figure}[!h]
%     \centering
%     \subfigure[Push button vertically with the gripper tip.]{%
%     \includegraphics[width=0.98\linewidth]{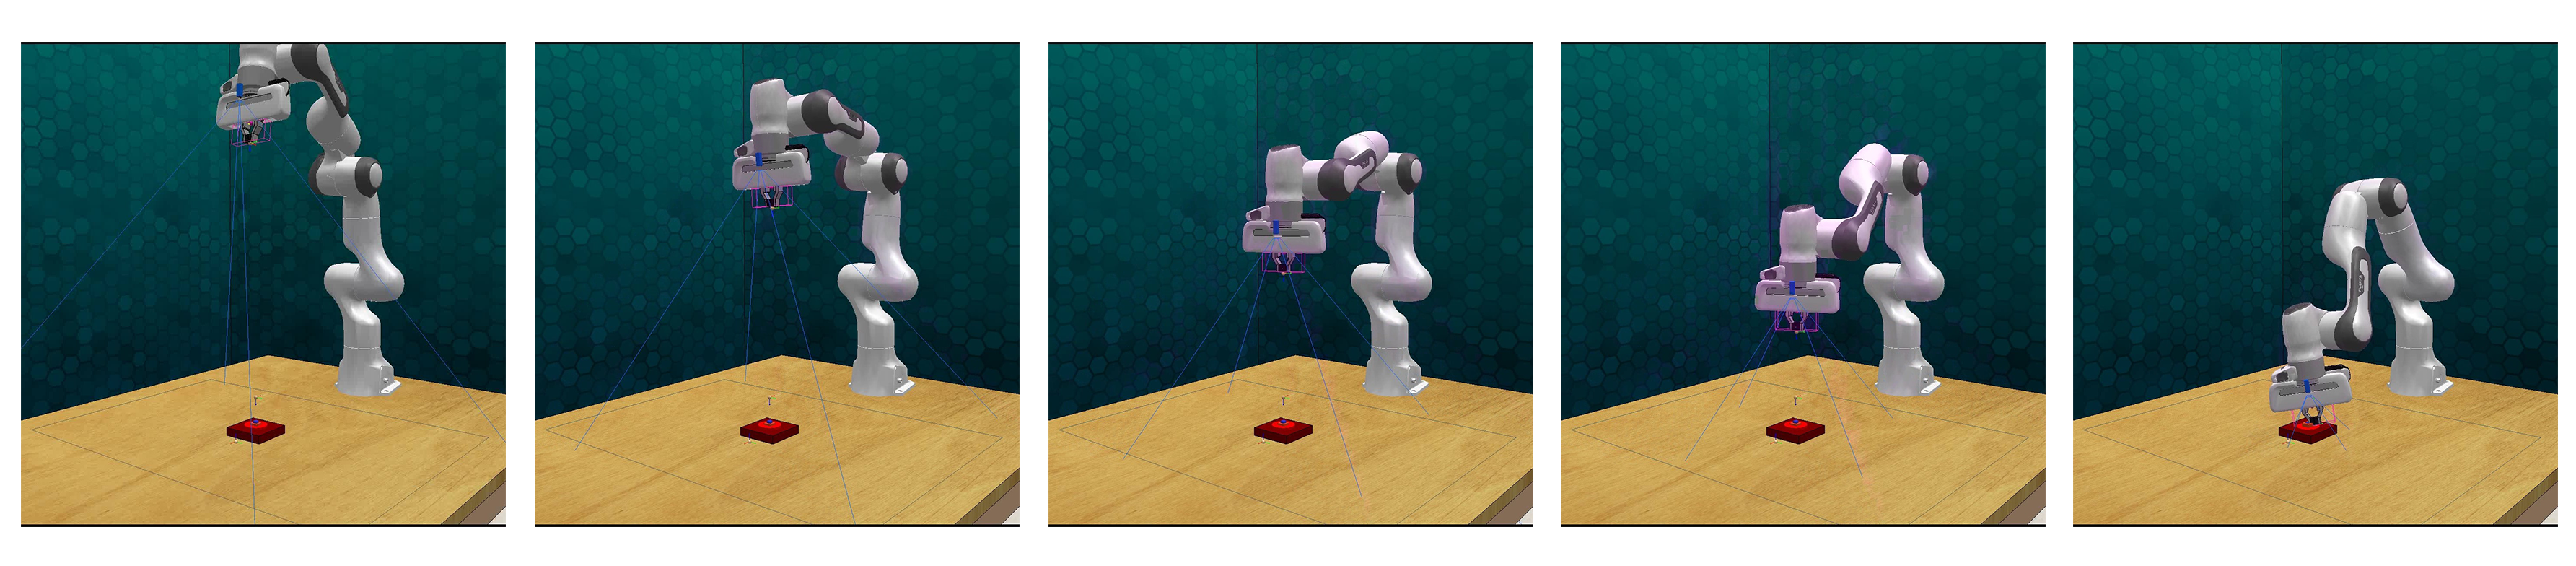}\label{5a}
%     }
%     \\
%     \subfigure[Push button horizontally with the gripper side.]{%
%     \includegraphics[width=0.98\linewidth]{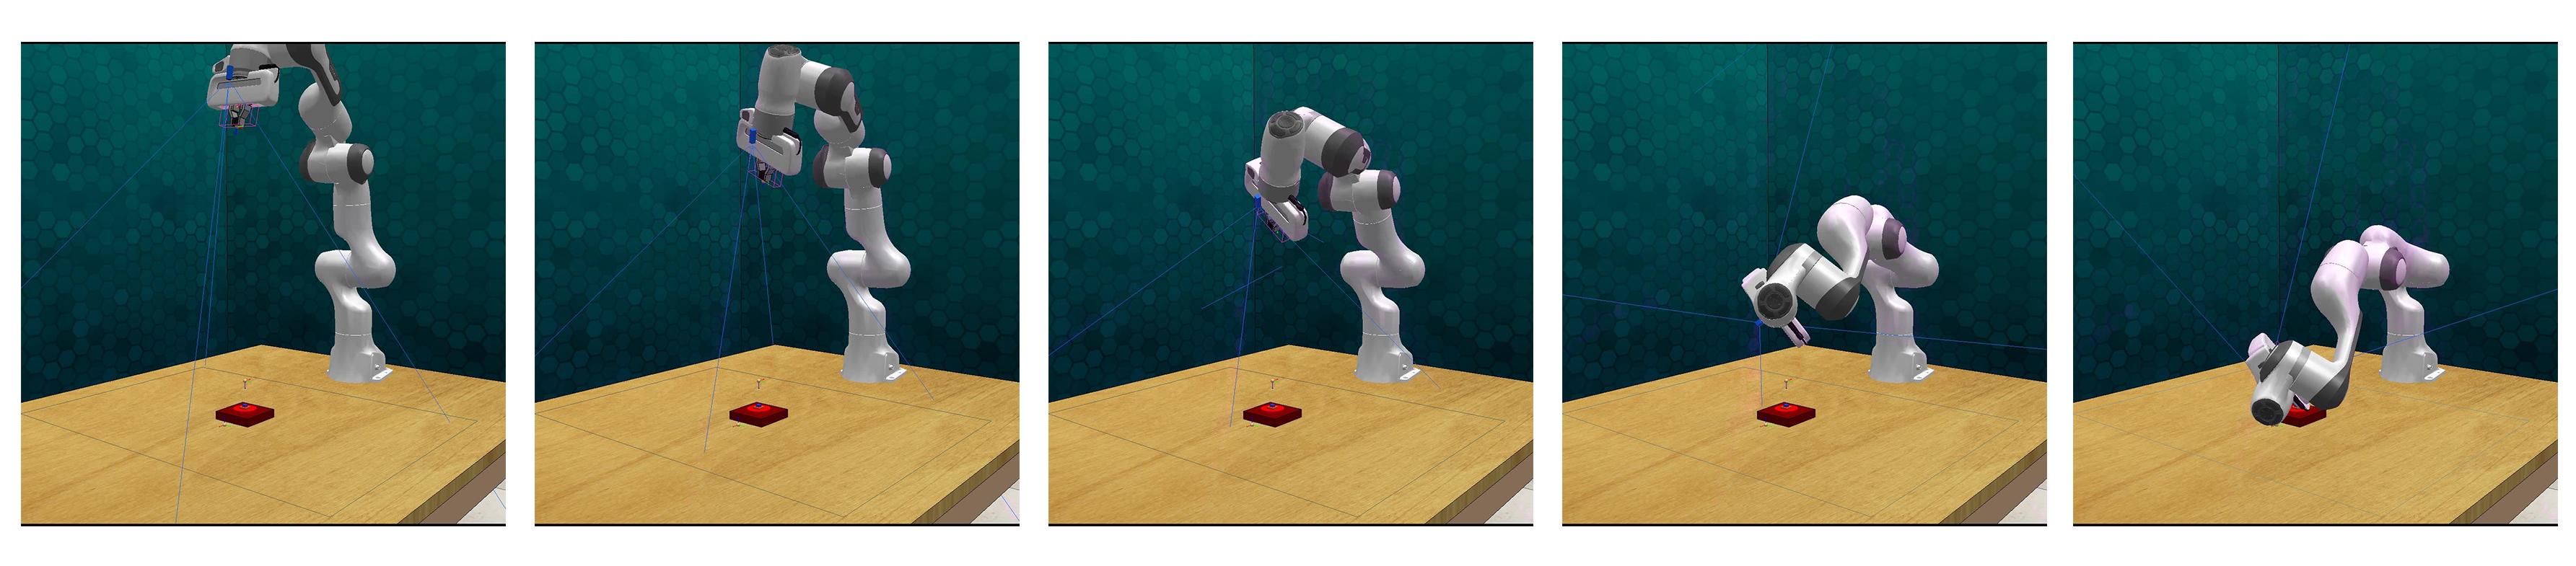}\label{5b}
%     }
%     \caption{Five frames of agent behaviors trained by the teachers with different preferences.}
%     \label{figure5} 
% \end{figure}

\section{A Showcase of Scoring}
Figure~\ref{figure-a1} shows an example that human scores in the Metaworld ButtonPress task. When the episode 480 of the training ended, the human teacher reviewed the 471-480 episodes via video playback and selected five episodes (the 471,474,475,477 and 479 episodes) to score.

\begin{figure}[!h]
\centering
\includegraphics[width=0.98\linewidth]{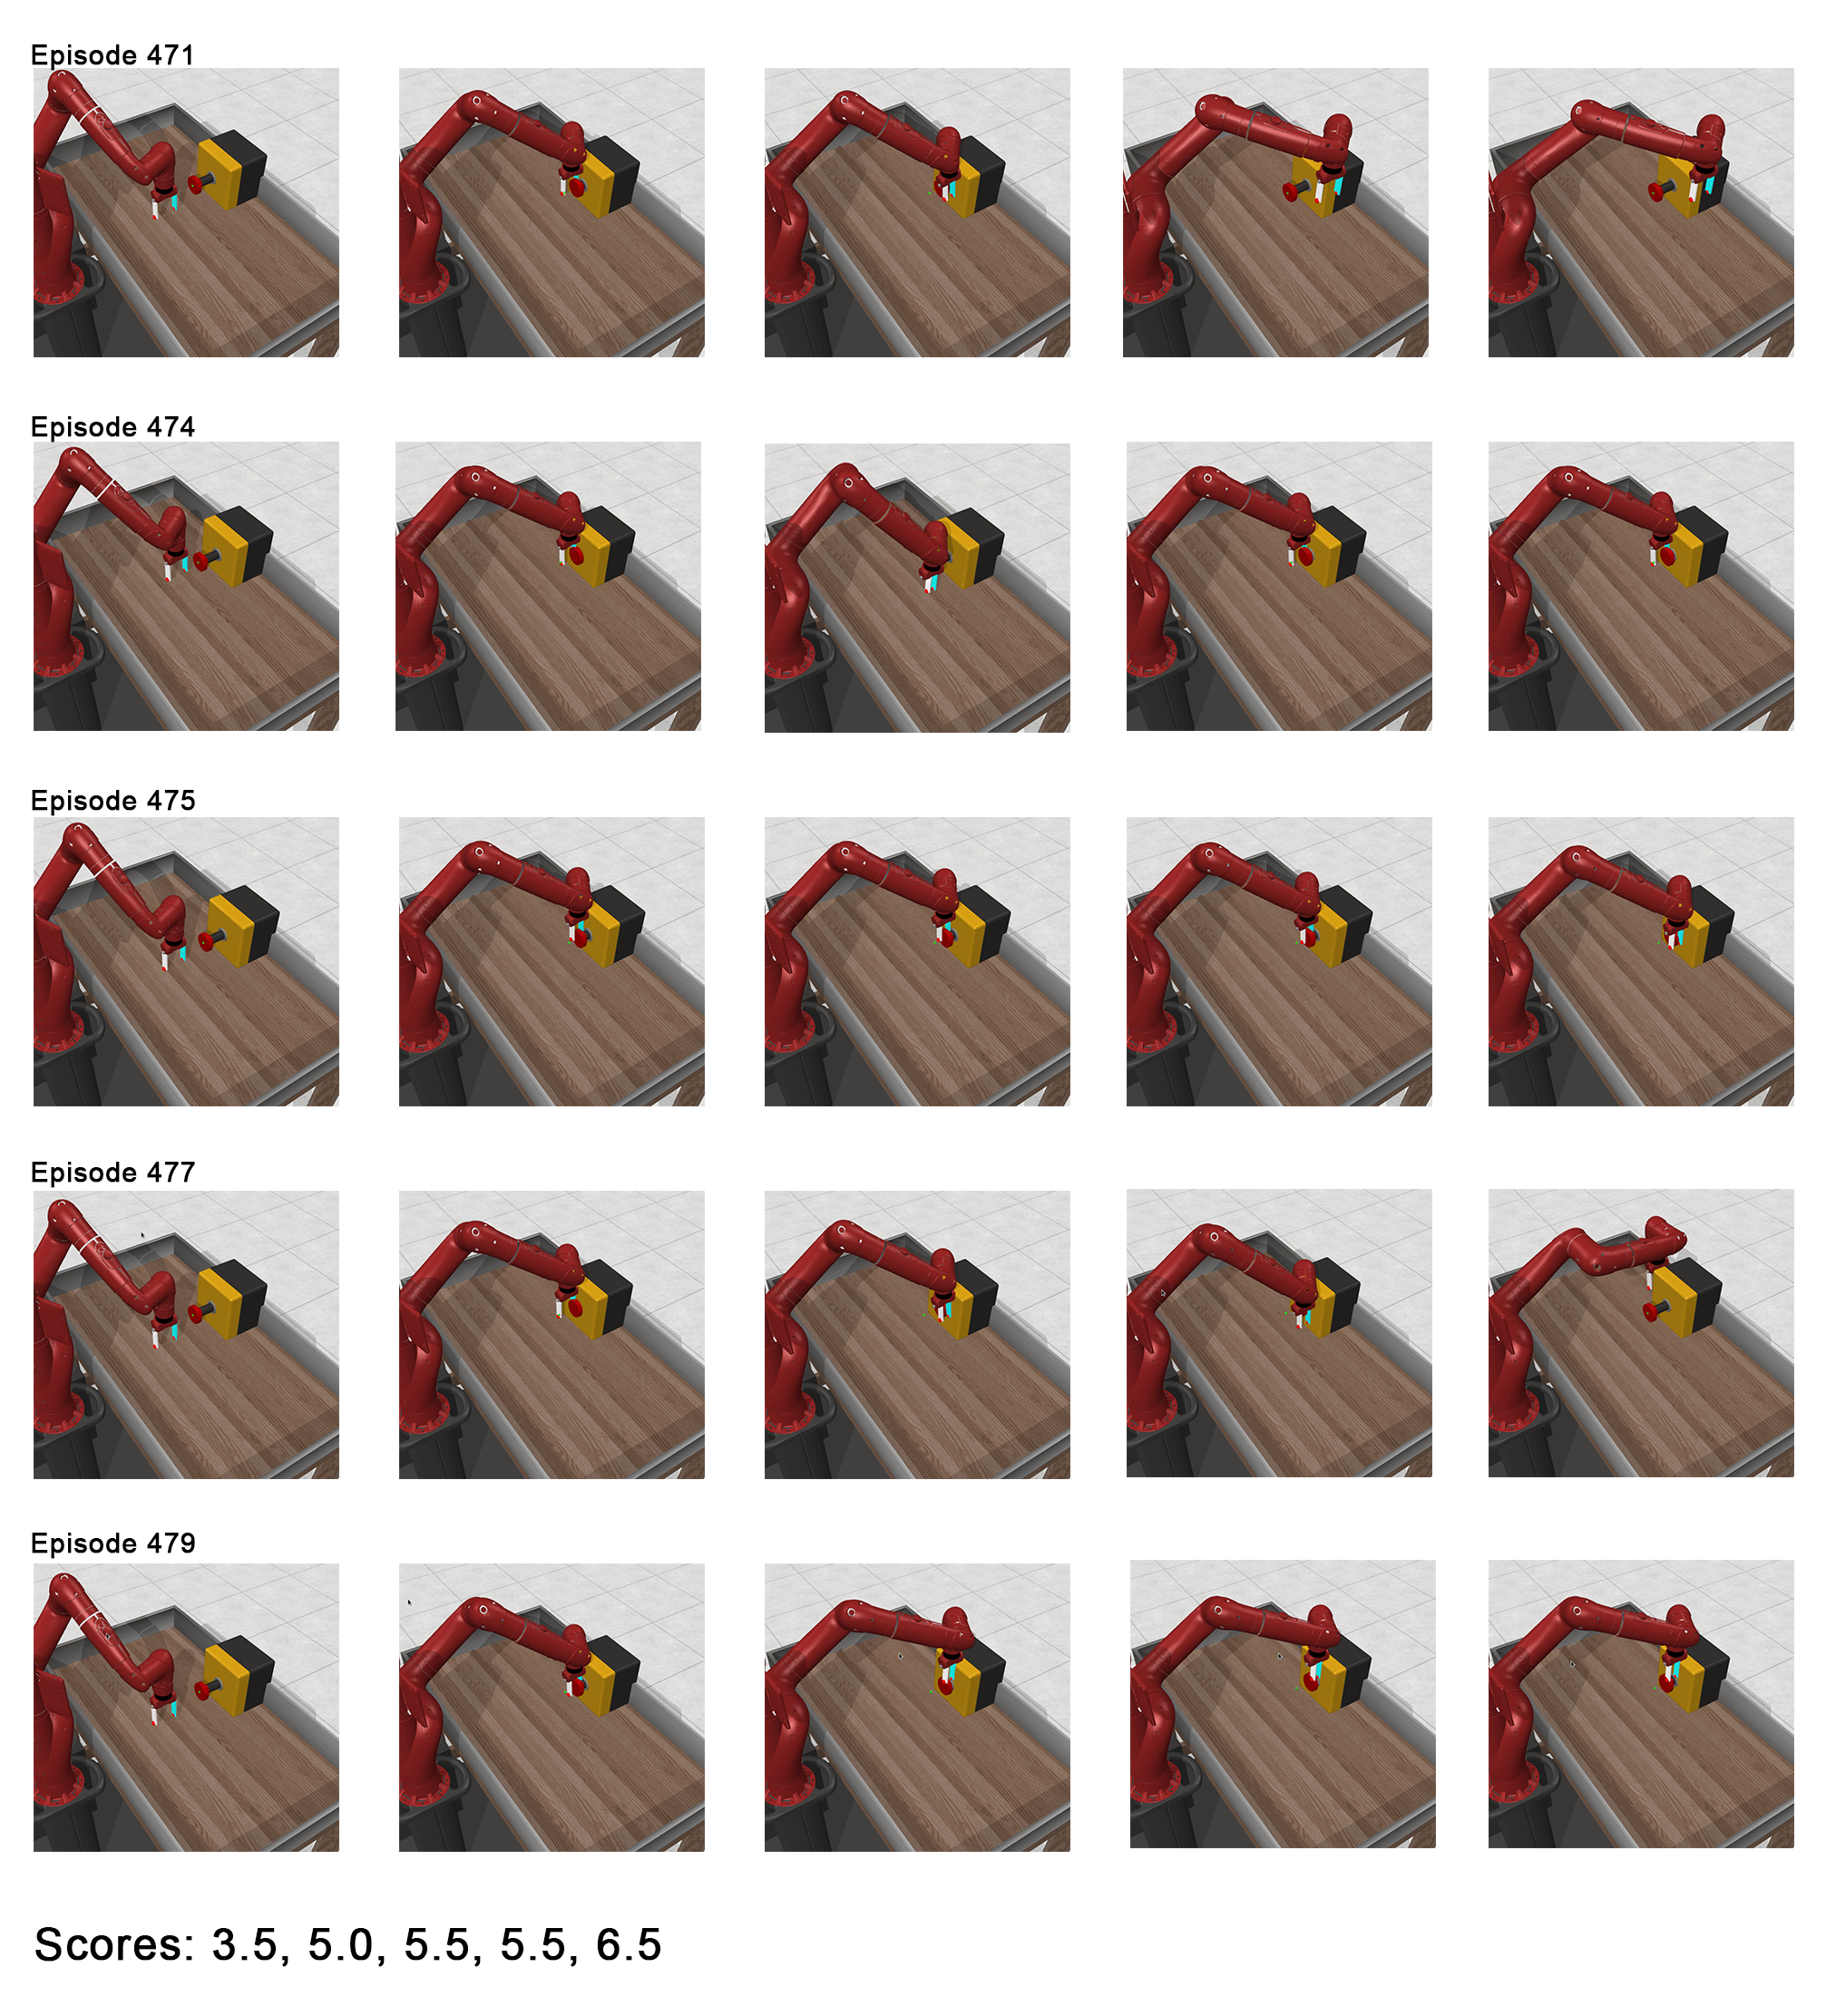}
\caption{Example of human teacher scoring trajectories in Metaworld Buttonpress task. In this task, the human teacher considers factors such as the speed at which the robotic arm presses the button, the degree to which the button is pressed, and how long it is held to be pressed. In this round of human scoring, the episodes 471, 474, 475, 477, and 479 are scored 3.5, 5.0, 5.5, 5.5, and 6.5 respectively.}
\label{figure-a1}
\end{figure}

\begin{figure} [!h]
    \centering
    \subfigure{%
    \includegraphics[height=4.2cm]{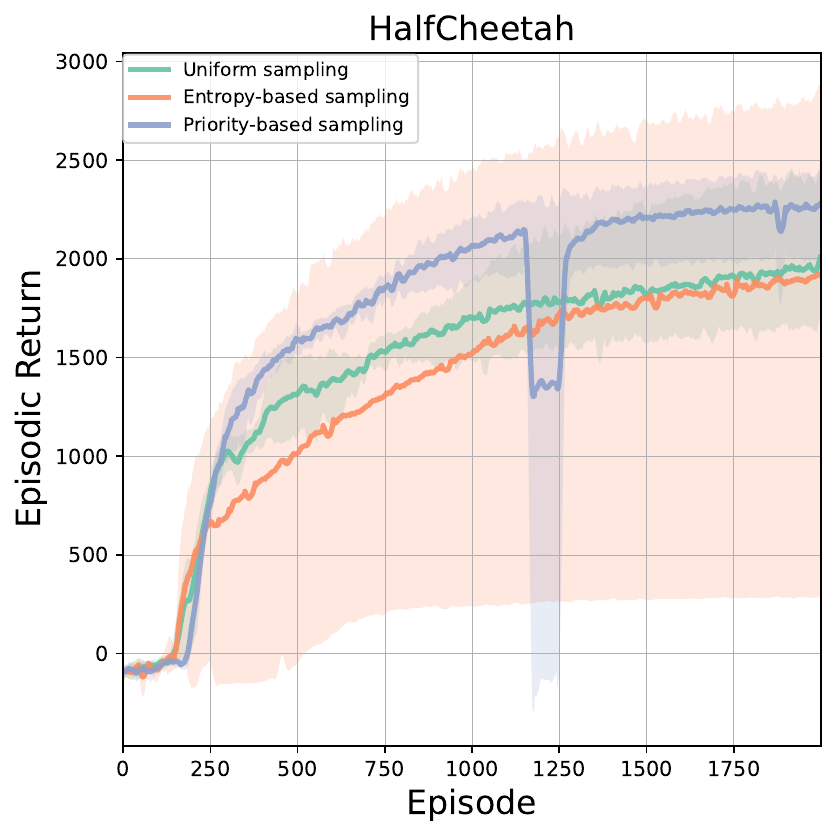}%\hspace*{1em}
    \includegraphics[height=4.2cm]{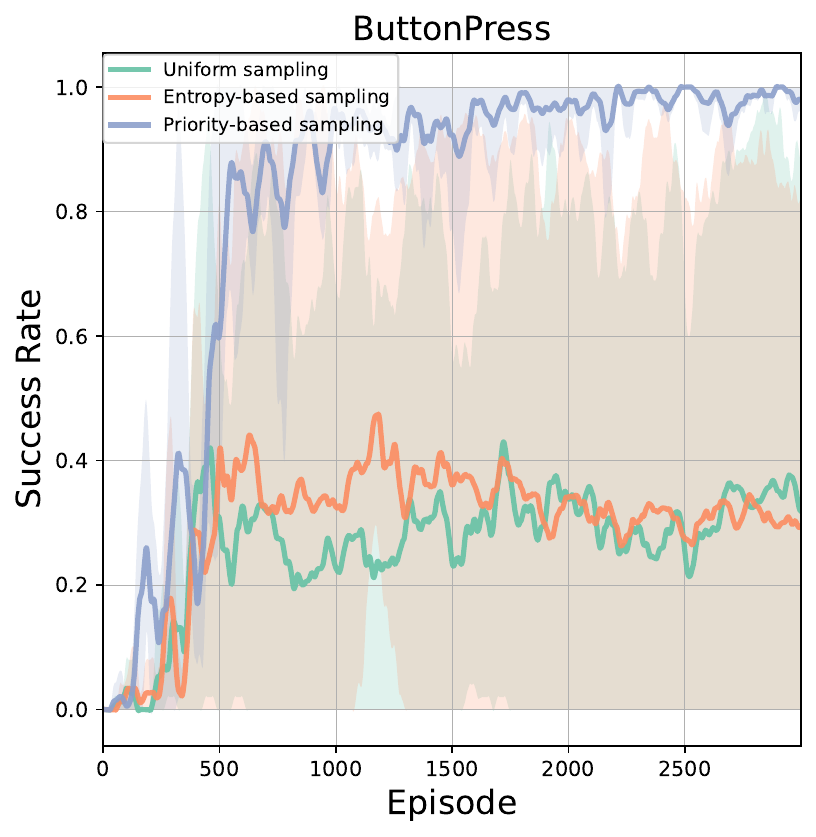}
    }
    \caption{Effects of sampling schemes with perfect correct scores. For HalfCheetah we score 250 trajecotries for each run; For ButtonPress we score 500 trajectoreis for each run.}
    \label{figure-a2} 
\end{figure}

\section{Effects of Sampling Methods}
In the Ablation study in the main paper, we have shown the effects of different sampling methods with noisy scores in HalfCheetah and PushButton tasks. In Figure~\ref{figure-a2}, we show the learning curves of our approach with these sampling methods with perfect correct scores generated by ground true reward. We can see that when using the perfect correct scores, in HalfCheetah, using uniform sampling and entropy-based sampling can approach the performance of using priority-based sampling. But in the more difficult task ButtonPress, using priority-based sampling still significantly outperforms the other two sampling methods. Overall, sampling by score-related priorities is better than sampling randomly or by entropy.
